# Supplementary material for: Few-mode Field Quantization of Arbitrary Electromagnetic Spectral Densities
Source: arXiv:2008.00349 ancillary file (2020-08-01)
Supplement: Supplementary file 1 [file supplemental.pdf]

# Supplemental Material
# Few-mode Field Quantization of Arbitrary Electromagnetic Spectral Densities

Ivan Medina,[1] Francisco J. García-Vidal,[2,3] Antonio I. Fernández-Domínguez,[2,*] and Johannes Feist[2,†]

[1]*Centro de Ciências Naturais e Humanas, Universidade Federal do ABC, 09210-170, Santo André, São Paulo, Brazil*
[2]*Departamento de Física Teórica de la Materia Condensada and Condensed Matter Physics Center (IFIMAC), Universidad Autónoma de Madrid, E-28049 Madrid, Spain*
[3]*Donostia International Physics Center (DIPC), E-20018 Donostia/San Sebastián, Spain*

## POSITIVITY OF $J_{\mathrm{mod}}(\omega)$

Here, we show that $J_{\mathrm{mod}}(\omega)$ is non-negative for all $\omega$. To do so, we rewrite Eq. (6) in the main text in the following way

$$J_{\mathrm{mod}}(\omega) = \frac{1}{\pi}\,\mathrm{Im}\left(\vec{g}^{\,T}\frac{1}{\Omega - i\sum_{j=1}^{N}\vec{y}_j\vec{y}_j^{\,T}}\vec{g}\right), \tag{1}$$

where $\Omega$ is a real symmetric $N\times N$ matrix with elements $\Omega_{ij} = \omega_{ij} - \omega\delta_{ij}$ and $\vec{y}_j = \sqrt{\frac{\kappa_j}{2}}(\delta_{1j}, \delta_{2j}, \ldots, \delta_{Nj})^T$ is a real column vector. Then, with help of the identities (see lemmas 2 and 3 in Ref. [1] for the proof),

$$\det(A - \vec{x}\vec{v}^{\,T}) = (1 - \vec{x}^{\,T}A^{-1}\vec{v})\det(A), \tag{2}$$

$$\left|\frac{\det(A - \vec{x}\vec{v}^{\,T})}{\det(A - i\vec{v}\vec{v}^{\,T})}\right|^2 = 1 + \mathrm{Im}[(\vec{x} - i\vec{v})^T(A - i\vec{v}\vec{v}^{\,T})^{-1} \times (\vec{x} - i\vec{v})], \tag{3}$$

where $A$ is any real symmetric regular square matrix, and $\vec{v}$ and $\vec{x}$ are real column vectors, it is possible to rewrite Eq. (1) as

$$J_{mod}(\omega) = \frac{1}{\pi}\sum_{j=1}^{N}\left|\vec{g}^{\,T}\frac{1}{\Omega - i\sum_{j=1}^{N}\vec{y}_j\vec{y}_j^{\,T}}\vec{y}_j\right|^2, \tag{4}$$

which is clearly non-negative for any $\omega$.

## OTHER EXAMPLES

Here, we use our model to fit the spectral densities of some hybrid cavity systems recently reported in the literature [2–4], and give explicit expressions for the model spectral density in the case of up to four modes. Fig. 1(a) shows the Purcell factor $J(\omega)/J_0(\omega)$ for the system described in [2, 3], which is composed of a dimer made of two gold nano-rods placed on top of a nano-beam plasmonic crystal cavity. The gold dimer is assumed to be in free space with background refractive index of $n_i = 1$, and its dielectric response is given by a Drude model with plasma frequency $\omega_p = 1.26\times10^{16}\ \mathrm{s}^{-1}$ and collision rate $\gamma_p = 1.41\times10^{14}\ \mathrm{s}^{-1}$. The nano-beam is made of silicon nitride, with refractive index $n_i = 2.04$. The Purcell factor generated by this hybrid structure exhibits two asymmetric peaks with a Fano-type interference near $\hbar\omega = 1.6$ eV, as shown in Fig. 1(a). We can see that that the non-interacting model fit with 3 modes (light blue line) mostly fails to reproduce the spectrum in this frequency window. On the other hand, the fitting using our model (orange line) for the same number of modes, i.e.,

$$J_{\mathrm{mod}}(\omega) = \frac{1}{\pi}\mathrm{Im}\Bigg\{\frac{1}{\mathcal{C}(\omega)}\Big[(g_2\omega_{13} - g_1\omega_{23})^2 + g_3^2\left(\omega_{12}^2 - \Lambda_1(\omega)\Lambda_2(\omega)\right) + 2g_3g_2\left(\omega_{23}\Lambda_1(\omega) - \omega_{12}\omega_{13}\right) + 2g_3g_1\left(\omega_{13}\Lambda_2(\omega) - \omega_{12}\omega_{23}\right) - \left(g_2^2\Lambda_1(\omega) + g_1^2\Lambda_2(\omega) - 2g_1g_2\omega_{12}\right)\Lambda_3(\omega)\Big]\Bigg\} \tag{5}$$

where $\Lambda_j(\omega) = \omega_j - \omega - i\frac{\kappa_j}{2}$ and $\mathcal{C}(\omega) = \omega_{12}^2\Lambda_3(\omega) + \Lambda_2(\omega)\left(\omega_{13}^2 - \Lambda_1(\omega)\Lambda_3(\omega)\right) - 2\omega_{12}\omega_{13}\omega_{23} + \omega_{23}^2\Lambda_1(\omega)$, fully reproduces the "correct" Purcell Factor (thick black line).

Fig. 1(b) shows the Purcell factor for the system in Ref. [4]. The hybrid structure consists of plasmonic gold nano-cone antenna embedded in a Fabry-Perot cavity. The cavity is composed of a flat mirror and a curved mirror spaced by a distance $L = 559$ nm. The hybrid cavity-antenna structure generates a Purcell factor with two main

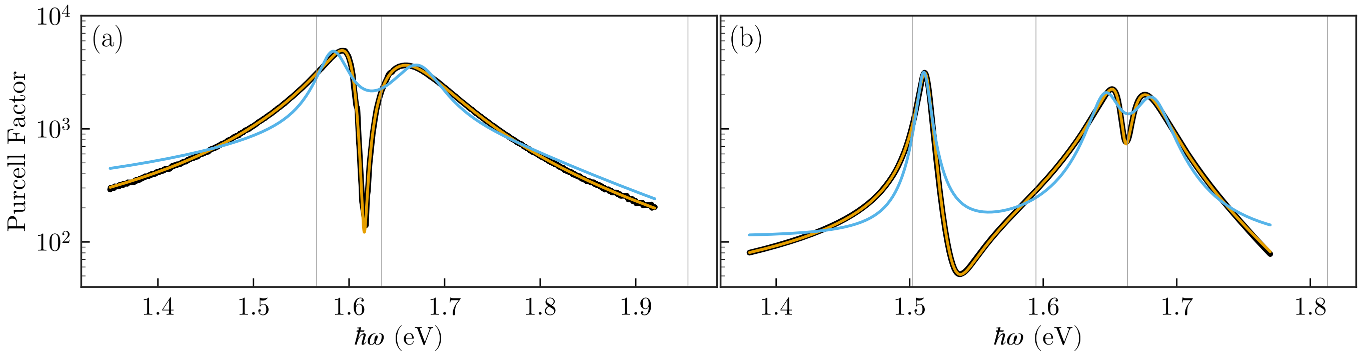


FIG. 1. (a) Numerical Purcell Factor $J(\omega)/J_0(\omega)$ (thick black line) for the gold dimer on the top of a nano-beam plasmonic crystal cavity [2, 3], and the fittings for the non-interacting model (light-blue line) and fit to the model $J_{\rm mod}(\omega)$ (orange line) using 3 modes. (b) Numerical Pucell Factor $J(\omega)/J_0(\omega)$ (thick black line) for the gold nano-cone antenna embedded in a Fabry-Perot cavity [4], and the fittings for the non-interacting model (light blue line) and fit to the model $J_{\rm mod}(\omega)$ (orange line) using 4 modes.

features: a "sharp peak" and a dip, near $\hbar\omega = 1.5$. These features result from constructive and destructive Fano-type interferences and are known as Fano peak and Fano dip, respectively. In Fig. 1(b), we see that the non-interacting model with 4 modes (light blue line) gives a reasonable fit for the Fano peak, but fails to reproduce the Fano dip and most of the rest of the spectrum. However, we see again that our model (orange line) with the same number of modes, i.e.,

$$
\begin{aligned}
J_{\rm mod}(\omega) = \frac{1}{\pi}\,{\rm Im}\Bigg\{ \frac{1}{\mathcal{C}(\omega)} \Big[ & 2g_3^2\omega_{12}\omega_{14}\omega_{24} - 2g_1g_3\omega_{14}\omega_{23}\omega_{24} + 2g_1g_3\omega_{13}\omega_{24}^2 - 2g_1g_3\omega_{12}\omega_{24}\omega_{34} + 2g_1^2\omega_{23}\omega_{24}\omega_{34} \\
& - g_3^2\omega_{24}^2\Lambda_1(\omega) - g_3^2\omega_{14}^2\Lambda_2(\omega) + 2g_1g_3\omega_{14}\omega_{34}\Lambda_2(\omega) - g_1^2\omega_{34}^2\Lambda_2(\omega) - g_1^2\omega_{24}^2\Lambda_3(\omega) \\
& - g_4^2\left[-2\omega_{12}\omega_{13}\omega_{23} + \omega_{23}^2\Lambda_1(\omega) + \omega_{12}^2\Lambda_3(\omega) + \Lambda_2(\omega)\left(\omega_{13}^2 - \Lambda_1(\omega)\Lambda_3(\omega)\right)\right] \\
& + 2g_4g_3\left[-\omega_{12}\left(\omega_{14}\omega_{23} + \omega_{13}\omega_{24}\right) + \omega_{12}^2\omega_{34} + \omega_{23}\omega_{24}\Lambda_1(\omega) + \left(\omega_{13}\omega_{14} - \omega_{34}\Lambda_1(\omega)\right)\Lambda_2(\omega)\right] \\
& + 2g_4g_2\left[\omega_{13}^2\omega_{24} - \omega_{13}\left(\omega_{14}\omega_{23} + \omega_{12}\omega_{34}\right) + \omega_{23}\omega_{34}\Lambda_1(\omega) + \left(\omega_{12}\omega_{14} - \omega_{24}\Lambda_1(\omega)\right)\Lambda_3(\omega)\right] \\
& + 2g_4g_1\left[\omega_{13}\left(\omega_{34}\Lambda_2(\omega) - \omega_{23}\omega_{24}\right) + \omega_{12}\left(\omega_{24}\Lambda_3(\omega) - \omega_{23}\omega_{34}\right) + \omega_{14}\left(\omega_{23}^2 - \Lambda_2(\omega)\Lambda_3(\omega)\right)\right] \\
& + 2g_1g_3\left[\left(\omega_{12}\omega_{23} - \omega_{13}\Lambda_2(\omega)\right) + g_3^2\left(\Lambda_1(\omega)\Lambda_2(\omega) - \omega_{12}^2\right) + g_1^2\left(\Lambda_2(\omega)\Lambda_3(\omega) - \omega_{23}^2\right)\right]\Lambda_4(\omega) \\
& - g_2^2\left[-2\omega_{13}\omega_{14}\omega_{34} + \omega_{34}^2\Lambda_1(\omega) + \omega_{13}^2\Lambda_4(\omega) + \Lambda_3(\omega)\left(\omega_{14}^2 - \Lambda_1[\omega]\Lambda_4(\omega)\right)\right] \\
& + 2g_2g_3\left[\omega_{14}^2\omega_{23} - \omega_{14}\left(\omega_{13}\omega_{24} + \omega_{12}\omega_{34}\right) + \omega_{24}\omega_{34}\Lambda_1(\omega) + \left(\omega_{12}\omega_{13} - \omega_{23}\Lambda_1(\omega)\right)\Lambda_4(\omega)\right] \\
& + 2g_2g_1\left[\omega_{14}\left(\omega_{24}\Lambda_3(\omega) - \omega_{23}\omega_{34}\right) + \omega_{13}\left(\omega_{23}\Lambda_4(\omega) - \omega_{24}\omega_{34}\right) + \omega_{12}\left(\omega_{34}^2 - \Lambda_3(\omega)\Lambda_4(\omega)\right)\right] \Big] \Bigg\},
\end{aligned}
\tag{6}
$$

with

$$
\begin{aligned}
\mathcal{C}(\omega) = & \omega_{12}^2\omega_{34}^2 + 2\omega_{23}\omega_{24}\omega_{34}\Lambda_1(\omega) - \omega_{34}^2\Lambda_1(\omega)\Lambda_2(\omega) - \omega_{24}^2\Lambda_1(\omega)\Lambda_3(\omega) + \omega_{14}^2\left(\omega_{23}^2 - \Lambda_2(\omega)\Lambda_3(\omega)\right) \\
& + 2\omega_{14}\left[\omega_{13}\left(\omega_{34}\Lambda_2(\omega) - \omega_{23}\omega_{24}\right) + \omega_{12}\left(\omega_{24}\Lambda_3(\omega) - \omega_{23}\omega_{34}\right)\right] - \omega_{23}^2\Lambda_1(\omega)\Lambda_4(\omega) + \\
& - \left(\omega_{12}^2 - \Lambda_1(\omega)\Lambda_2(\omega)\right)\Lambda_3(\omega)\Lambda_4(\omega) + 2\omega_{12}\omega_{13}\left(\omega_{23}\Lambda_4(\omega) - \omega_{24}\omega_{34}\right) + \omega_{13}^2\left(\omega_{24}^2 - \Lambda_2(\omega)\Lambda_4(\omega)\right),
\end{aligned}
\tag{7}
$$

gives a fit in full agreement with the "correct" Purcell Factor (thick black line).

Finally, in Table I and Table II we show the fitting parameters used in Fig. 1(a) and Fig. 1(b). Here, $\omega_{ij}$ and $\kappa_j$ are in eV and $\tilde{g}_j = g_j \times 10^7 \mu^{-1}$. It is worth remarking that although the $\omega_{ij}$ is within the frequency window, some of the eigenmodes (obtained by diagonalizing $\omega_{ij}$), shown in the vertical grey lines in Fig. 1, are outside of this window. This happens exactly because we have just a limited window of frequencies available in these cases.

| - | $\tilde{g}_1$ | $\tilde{g}_2$ | $\tilde{g}_3$ | $\omega_{12}$ | $\omega_{13}$ | $\omega_{23}$ | $\kappa_1$ | $\kappa_2$ | $\kappa_3$ | $\omega_1$ | $\omega_2$ | $\omega_3$ |
|---|---|---|---|---|---|---|---|---|---|---|---|---|
| Model | 0.259 | 1.224 | 0.079 | 0.130 | 0.010 | -0.030 | 1.570 | 0.095 | 4e-3 | 1.900 | 1.644 | 1.613 |
| NI Model | 0.959 | 0.659 | -0.559 | 0 | 0 | 0 | 0.354 | 0.056 | 0.033 | 1.683 | 1.671 | 1.583 |

TABLE I. Fitting parameters for the plots of Fig. 1(a).

| - | $\tilde{g}_1$ | $\tilde{g}_2$ | $\tilde{g}_3$ | $\tilde{g}_4$ | $\omega_{12}$ | $\omega_{13}$ | $\omega_{14}$ | $\omega_{23}$ | $\omega_{24}$ | $\omega_{34}$ | $\kappa_1$ | $\kappa_2$ | $\kappa_3$ | $\kappa_4$ | $\omega_1$ | $\omega_2$ | $\omega_3$ | $\omega_4$ |
|---|---|---|---|---|---|---|---|---|---|---|---|---|---|---|---|---|---|---|
| Model | 0.121 | 0.558 | 0.224 | 0.101 | -0.105 | -0.041 | -0.015 | 0.007 | -0.031 | -0.018 | 0.928 | 4.4e-3 | 0.005 | 0.003 | 1.726 | 1.654 | 1.668 | 1.522 |
| NI Model | 0.320 | 0.293 | 0.385 | 0.0.25 | 0 | 0 | 0 | 0 | 0 | 0 | 0.023 | 0.019 | 0.122 | 0.010 | 1.680 | 1.647 | 1.668 | 1.510 |

TABLE II. Fitting parameters for the plots of Fig. 1(b).

* a.fernandez-dominguez@uam.es
† johannes.feist@uam.es

[1] S. Glutsch, Optical Absorption of the Fano Model: General Case of Many Resonances and Many Continua, Phys. Rev. B **66**, 075310 (2002).

[2] M. Kamandar Dezfouli and S. Hughes, Quantum Optics Model of Surface-Enhanced Raman Spectroscopy for Arbitrarily Shaped Plasmonic Resonators, ACS Photonics **4**, 1245 (2017).

[3] S. Franke, S. Hughes, M. Kamandar Dezfouli, P. T. Kristensen, K. Busch, A. Knorr, and M. Richter, Quantization of Quasinormal Modes for Open Cavities and Plasmonic Cavity Quantum Electrodynamics, Phys. Rev. Lett. **122**, 213901 (2019).

[4] B. Gurlek, V. Sandoghdar, and D. Martín-Cano, Manipulation of Quenching in Nanoantenna–Emitter Systems Enabled by External Detuned Cavities: A Path to Enhance Strong-Coupling, ACS Photonics **5**, 456 (2018).
